# Supplementary material for: Measurements of Differential Cross Sections of Inclusive $\pi^0$ and $K^0_S$ Production in $e^{+}e^{-}$ Annihilation at Energies from 2.2324 to 3.6710 GeV
Source: arXiv:2211.11253 source file (2023-06-07)
Supplement: Supplementary file 1 [file Inclusive_pi0_Ks_Supplemental_material_SP.pdf]

# Measurements of Differential Cross Sections of Inclusive $\pi^0$ and $K_S^0$ Production in $e^+e^-$ Annihilation at Energies from 2.2324 to 3.6710 GeV: Supplemental material

M. Ablikim[1], M. N. Achasov[12,b], P. Adlarson[72], M. Albrecht[4], R. Aliberti[33], A. Amoroso[71A,71C], M. R. An[37], An[68,55], Y. Bai[54], O. Bakina[34], R. Baldini Ferroli[27A], I. Balossino[28A], Y. Ban[44,g], V. Batozskaya[1,42], D. Becker[33], K. Begzsuren[30], N. Berger[33], M. Bertani[27A], D. Bettoni[28A], F. Bianchi[71A,71C], E. Bianco[71A,71C], J. Bloms[65], A. Bortone[71A,71C], I. Boyko[34], R. A. Briere[5], A. Brueggemann[65], H. Cai[73], X. Cai[1,55], A. Calcaterra[27A], G. F. Cao[1,60], N. Cao[1,60], S. A. Cetin[59A], J. F. Chang[1,55], W. L. Chang[1,60], G. R. Che[41], G. Chelkov[34,a], C. Chen[41], Chao Chen[52], G. Chen[1], H. S. Chen[1,60], M. L. Chen[1,55], S. J. Chen[40], S. M. Chen[58], T. Chen[1,60], X. R. Chen[29,60], X. T. Chen[1,60], Y. B. Chen[1,55], Z. J. Chen[24,h], W. S. Cheng[71C], S. K. Choi [52], X. Chu[41], G. Cibinetto[28A], F. Cossio[71C], J. J. Cui[47], H. L. Dai[1,55], J. P. Dai[76], A. Dbeyssi[18], R. E. de Boer[4], D. Dedovich[34], Z. Y. Deng[1], A. Denig[33], I. Denysenko[34], M. Destefanis[71A,71C], F. De Mori[71A,71C], Y. Ding[38], Y. Ding[32], J. Dong[1,55], L. Y. Dong[1,60], M. Y. Dong[1,55,60], X. Dong[73], S. X. Du[78], Z. H. Duan[40], P. Egorov[34,a], Y. L. Fan[73], J. Fang[1,55], S. S. Fang[1,60], W. X. Fang[1], Y. Fang[1], R. Farinelli[28A], L. Fava[71B,71C], F. Feldbauer[4], G. Felici[27A], C. Feng[68,55], J. H. Feng[56], K Fischer[66], M. Fritsch[4], C. Fritzsch[65], C. D. Fu[1], H. Gao[60], X. L. Gao[68,m], Y. N. Gao[44,g], Yang Gao[68,55], S. Garbolino[71C], I. Garzia[28A,28B], P. T. Ge[73], Z. W. Ge[40], C. Geng[56], E. M. Gersabeck[64], A Gilman[66], K. Goetzen[13], L. Gong[38], W. X. Gong[1,55], W. Gradl[33], M. Greco[71A,71C], L. M. Gu[40], M. H. Gu[1,55], Y. T. Gu[15], C. Y Guan[1,60], A. Guo[29,60], L. B. Guo[39], R. P. Guo[46], Y. P. Guo[11,f], A. Guskov[34,a], W. Y. Han[37], X. Hao[19], F. A. Harris[62], K. K. He[52], K. L. He[1,60], F. H. Heinsius[4], C. H. Heinz[33], Y. K. Heng[1,55,60], C. Herold[57], G. Y. Hou[1,60], Y. R. Hou[60], Z. L. Hou[1], H. M. Hu[1,60], J. F. Hu[53,i], T. Hu[1,55,60], Y. Hu[1], G. S. Huang[68,55], K. X. Huang[56], L. Huang[29,60], X. T. Huang[47], Y. P. Huang[1], Z. Huang[44,g], T. Hussain[70], N. Hüsken[26,33], W. Imoehl[26], M. Irshad[68,55], J. Jackson[26], S. Jaeger[4], S. Janchiv[30], E. Jang[52], J. H. Jeong[52], Ji[1], P. Ji[19], X. B. Ji[1,60], X. L. Ji[1,55], Y. Y. Ji[47], Z. K. Jia[68,55], P. C. Jiang[44,g], S. S. Jiang[37], X. S. Jiang[1,55,60], Y. Jiang[60], J. B. Jiao[47], Z. Jiao[22], S. Jin[40], Y. Jin[63], M. Jing[1,60], T. Johansson[72], S. Kabana[31], N. Kalantar-Nayestanaki[61], X. L. Kang[9], X. S. Kang[38], R. Kappert[61], M. Kavatsyuk[61], B. C. Ke[78], I. K. Keshk[4], A. Khoukaz[65], R. Kiuchi[1], R. Kliemt[13], L. Koch[35], O. B. Kolcu[59A], B. Kopf[4], M. Kuemmel[4], M. Kuessner[4], A. Kupsc[42,72], W. Kühn[35], J. J. Lane[64], J. S. Lange[35], P. Larin[18], A. Lavania[25], L. Lavezzi[71A,71C], T. T. Lei[68,k], Z. H. Lei[68,55], H. Leithoff[33], M. Lellmann[33], T. Lenz[33], C. Li[41], C. Li[45], C. H. Li[37], Cheng Li[68,55], D. M. Li[78], F. Li[1,55], G. Li[1], H. Li[49], H. Li[68,55], H. B. Li[1,60], H. J. Li[19], H. N. Li[53,i], J. Li[4], J. S. Li[56], J. W. Li[47], Ke Li[1], L. J Li[1,60], L. K. Li[1], Lei Li[3], M. H. Li[41], P. R. Li[36,j,k], S. X. Li[11], S. Y. Li[58], T. Li[47], W. D. Li[1,60], W. G. Li[1], X. H. Li[68,55], X. L. Li[47], Xiaoyu Li[1,60], Y. G. Li[44,g], Z. X. Li[15], Z. Y. Li[56], C. Liang[40], H. Liang[32], H. Liang[1,60], H. Liang[68,55], Y. F. Liang[51], Y. T. Liang[29,60], G. R. Liao[14], L. Z. Liao[47], J. Libby[25], A. Limphirat[57], C. X. Lin[56], D. X. Lin[29,60], T. Lin[1], B. J. Liu[1], C. Liu[32], C. X. Liu[1], D. Liu[18,68], F. H. Liu[50], Fang Liu[1], Feng Liu[6], G. M. Liu[53,i], H. Liu[36,j,k], H. B. Liu[15], H. M. Liu[1,60], Huanhuan Liu[1], Huihui Liu[20], J. B. Liu[68,55], J. L. Liu[69], J. Y. Liu[1,60], K. Liu[1], K. Y. Liu[38], Ke Liu[21], L. Liu[68,55], Lu Liu[41], M. H. Liu[11,f], P. L. Liu[1], Liu[60], S. B. Liu[68,55], T. Liu[11,f], W. K. Liu[41], W. M. Liu[68,55], X. Liu[36,j,k], Y. Liu[36,j,k], Y. B. Liu[41], Z. A. Liu[1,55,60], Z. Liu[47], X. C. Lou[1,55,60], F. X. Lu[56], H. J. Lu[22], J. G. Lu[1,55], X. L. Lu[1], Y. Lu[7], Y. P. Lu[1,55], Z. H. Lu[1,60], C. L. Luo[39], M. X. Luo[77], T. Luo[11,f], X. L. Luo[1,55], X. R. Lyu[60], Y. F. Lyu[41], F. C. Ma[38], H. L. Ma[1], L. L. Ma[47], M. M. Ma[1,60], M. Ma[1], R. Ma[1,60], R. T. Ma[60], X. Y. Ma[1,55], Y. Ma[44,g], F. E. Maas[18], M. Maggiora[71A,71C], S. Maldaner[4], S. Malde[66], A. Malik[70], A. Mangoni[27B], Y. J. Mao[44,g], Z. P. Mao[1], S. Marcello[71A,71C], Z. X. Meng[63], J. G. Messchendorp[13,61], G. Mezzadri[28A], H. Miao[1,60], T. J. Min[40], R. E. Mitchell[26], X. H. Mo[1,55,60], N. Yu. Muchnoi[12,b], Y. Nefedov[34], F. Nerling[18,d], I. B. Nikolaev[12,b], Z. Ning[1,55], S. Nisar[10,l], Y. Niu [47], S. L. Olsen[60], Ouyang[1,55,60], S. Pacetti[27B,27C], X. Pan[11,f], Y. Pan[54], A. Pathak[32], Y. P. Pei[68,55], M. Pelizaeus[4], H. P. Peng[68,55], K. Peters[13,d], J. L. Ping[39], R. G. Ping[1,60], S. Plura[33], S. Pogodin[34], V. Prasad[68,55], F. Z. Qi[1], H. Qi[68,55], H. R. Qi[58], M. Qi[40], T. Y. Qi[11,f], S. Qian[1,55], W. B. Qian[60], Z. Qian[56], C. F. Qiao[60], J. J. Qin[69], L. Qin[14], X. P. Qin[11,f], X. S. Qin[47], Z. H. Qin[1,55], J. F. Qiu[1], S. Qu[58], K. H. Rashid[70], C. F. Redmer[33], K. J. Ren[37], A. Rivetti[71C], V. Rodin[61], M. Rolo[71C], G. Rong[1,60], Ch. Rosner[18], S. N. Ruan[41], A. Sarantsev[34,c], Y. Schelhaas[33], C. Schnier[4], K. Schoenning[72], M. Scodeggio[28A,28B], K. Y. Shan[11,f], W. Shan[23], X. Y. Shan[68,55], J. F. Shangguan[52], L. G. Shao[1,60], M. Shao[68,55], C. P. Shen[11,f], H. F. Shen[1,60], W. H. Shen[60], X. Y. Shen[1,60], B. A. Shi[60], H. C. Shi[68,55], J. Y. Shi[1], Q. Q. Shi[52], R. S. Shi[1,60], X. Shi[1,55], J. J. Song[19], W. M. Song[32,1], Y. X. Song[44,g], S. Sosio[71A,71C], S. Spataro[71A,71C], F. Stieler[33], P. P. Su[52], Y. J. Su[60], G. X. Sun[1], H. Sun[60], H. K. Sun[1], J. F. Sun[19], L. Sun[73], S. S. Sun[1,60], T. Sun[1,60], W. Y. Sun[32], Y. J. Sun[68,55], Y. Z. Sun[1], Z. T. Sun[47], Y. H. Tan[73], Y. X. Tan[68,55], C. J. Tang[51], G. Y. Tang[1], J. Tang[56], L. Y Tao[69], T. Tao[24,h], M. Tat[66], J. X. Teng[68,55], V. Thoren[72], W. H. Tian[49], Y. Tian[29,60], I. Uman[59B], B. Wang[68,55], B. Wang[1], B. L. Wang[60], C. W. Wang[40], D. Y. Wang[44,g], F. Wang[69], H. J. Wang[36,j,k], H. P. Wang[1,60], K. Wang[1,55], L. L. Wang[1], M. Wang[47], M. Z. Wang[44,g], Meng Wang[1,60], S. Wang[11,f], S. Wang[14], T. Wang[11,f], T. J. Wang[41], W. Wang[56], W. H. Wang[73], W. P. Wang[68,55], X. Wang[44,g], X. F. Wang[36,j,k], X. L. Wang[11,f], Y. Wang[58], Y. D. Wang[43], Y. F. Wang[1,55,60], Y. H. Wang[45], Y. Wang[1], Yaqian Wang[17,1], Z. Wang[1,55], Z. Y. Wang[1,60], Ziyi Wang[60], D. H. Wei[14], F. Weidner[65], S. P. Wen[1], D. J. White[64], U. Wiedner[4], G. Wilkinson[66], M. Wolke[72], L. Wollenberg[4], J. F. Wu[1,60], L. H. Wu[1], L. J. Wu[1,60], X. Wu[11,f], X. H. Wu[32], Y. Wu[68], Y. J Wu[29], Z. Wu[1,55], L. Xia[68,55], T. Xiang[44,g], D. Xiao[36,j,k], G. Y. Xiao[40], H. Xiao[11,f], S. Y. Xiao[1], Y. L. Xiao[11,f], Z. J. Xiao[39], C. Xie[40], X. H. Xie[44,g], Y. Xie[47], Y. G. Xie[1,55], Y. H. Xie[6], Z. P. Xie[68,55], T. Y. Xing[1,60], C. F. Xu[1,60], C. J. Xu[56], G. F. Xu[1], H. Y. Xu[63], J. Xu[16], X. P. Xu[52], Y. C. Xu[75], Z. P. Xu[40], F. Yan[11,f], L. Yan[11,f], W. B. Yan[68,55], W. C. Yan[78], H. J. Yang[48,e], H. L. Yang[32], H. X. Yang[1], Tao Yang[1], Y. F. Yang[41], Y. X. Yang[1,60], Yifan Yang[1,60], M. Ye[1,55], M. H. Ye[8], J. H. Yin[1], Z. Y. You[56], B. X. Yu[1,55,60], C. X. Yu[41], G. Yu[1,60], T. Yu[69], X. D. Yu[44,g], C. Z. Yuan[1,60], L. Yuan[2], S. C. Yuan[1], X. Yuan[1], Y. Yuan[1,60], Z. Y. Yuan[56], C. X. Yue[37], A. A. Zafar[70], F. R. Zeng[47], X. Zeng[6], Y. Zeng[24,h], X. Y. Zhai[32], Y. H. Zhan[56], A. Zhang[1,60], B. L. Zhang[1,60], B. X. Zhang[1], D. H. Zhang[41], G. Y. Zhang[19], H. Zhang[68], H. H. Zhang[56], H. H. Zhang[32], H. Zhang[1,55,60], H. Y. Zhang[1,55], J. L. Zhang[74], J. Zhang[39],

J. W. Zhang[1,55,60], J. X. Zhang[36,j,k], J. Y. Zhang[1], J. Z. Zhang[1,60], Jianyu Zhang[1,60], Jiawei Zhang[1,60], L. M. Zhang[58], L. Zhang[56], Lei Zhang[40], P. Zhang[1], Y. Zhang[37,78], Shuihan Zhang[1,60], Shulei Zhang[24,h], X. D. Zhang[43], X. M. Zhang[1], X. Y. Zhang[47], X. Y. Zhang[52], Y. Zhang[66], Y. T. Zhang[78], Y. H. Zhang[1,55], Yan Zhang[68,55], Yao Zhang[1], Z. H. Zhang[1], Z. L. Zhang[32], Z. Y. Zhang[41], Z. Y. Zhang[73], G. Zhao[1], J. Zhao[37], J. Y. Zhao[1,60], J. Z. Zhao[1,55], Lei Zhao[68,55], Ling Zhao[1], M. G. Zhao[41], S. J. Zhao[78], Y. B. Zhao[1,55], Y. X. Zhao[29,60], Z. G. Zhao[68,55], A. Zhemchugov[34,a], B. Zheng[69], J. P. Zheng[1,55], Y. H. Zheng[60], B. Zhong[39], C. Zhong[69], X. Zhong[56], H. Zhou[47], L. P. Zhou[1,60], X. Zhou[73], X. K. Zhou[60], X. R. Zhou[68,55], X. Y. Zhou[37], Y. Z. Zhou[11,f], J. Zhu[41], K. Zhu[1], K. J. Zhu[1,55,60], L. X. Zhu[60], S. H. Zhu[67], S. Zhu[40], T. J. Zhu[74], W. J. Zhu[11,f], Y. C. Zhu[68,55], Z. A. Zhu[1,60], J. H. Zou[1], J. Zu[68,55]

(BESIII Collaboration)

[1] *Institute of High Energy Physics, Beijing 100049, People's Republic of China*
[2] *Beihang University, Beijing 100191, People's Republic of China*
[3] *Beijing Institute of Petrochemical Technology, Beijing 102617, People's Republic of China*
[4] *Bochum Ruhr-University, D-44780 Bochum, Germany*
[5] *Carnegie Mellon University, Pittsburgh, Pennsylvania 15213, USA*
[6] *Central China Normal University, Wuhan 430079, People's Republic of China*
[7] *Central South University, Changsha 410083, People's Republic of China*
[8] *China Center of Advanced Science and Technology, Beijing 100190, People's Republic of China*
[9] *China University of Geosciences, Wuhan 430074, People's Republic of China*
[10] *COMSATS University Islamabad, Lahore Campus, Defence Road, Off Raiwind Road, 54000 Lahore, Pakistan*
[11] *Fudan University, Shanghai 200433, People's Republic of China*
[12] *G.I. Budker Institute of Nuclear Physics SB RAS (BINP), Novosibirsk 630090, Russia*
[13] *GSI Helmholtzcentre for Heavy Ion Research GmbH, D-64291 Darmstadt, Germany*
[14] *Guangxi Normal University, Guilin 541004, People's Republic of China*
[15] *Guangxi University, Nanning 530004, People's Republic of China*
[16] *Hangzhou Normal University, Hangzhou 310036, People's Republic of China*
[17] *Hebei University, Baoding 071002, People's Republic of China*
[18] *Helmholtz Institute Mainz, Staudinger Weg 18, D-55099 Mainz, Germany*
[19] *Henan Normal University, Xinxiang 453007, People's Republic of China*
[20] *Henan University of Science and Technology, Luoyang 471003, People's Republic of China*
[21] *Henan University of Technology, Zhengzhou 450001, People's Republic of China*
[22] *Huangshan College, Huangshan 245000, People's Republic of China*
[23] *Hunan Normal University, Changsha 410081, People's Republic of China*
[24] *Hunan University, Changsha 410082, People's Republic of China*
[25] *Indian Institute of Technology Madras, Chennai 600036, India*
[26] *Indiana University, Bloomington, Indiana 47405, USA*
[27] *INFN Laboratori Nazionali di Frascati , (A)INFN Laboratori Nazionali di Frascati, I-00044, Frascati, Italy; (B)INFN Sezione di Perugia, I-06100, Perugia, Italy; (C)University of Perugia, I-06100, Perugia, Italy*
[28] *INFN Sezione di Ferrara, (A)INFN Sezione di Ferrara, I-44122, Ferrara, Italy; (B)University of Ferrara, I-44122, Ferrara, Italy*
[29] *Institute of Modern Physics, Lanzhou 730000, People's Republic of China*
[30] *Institute of Physics and Technology, Peace Avenue 54B, Ulaanbaatar 13330, Mongolia*
[31] *Instituto de Alta Investigacion, Universidad de Tarapaca, Casilla 7D, Arica, Chile*
[32] *Jilin University, Changchun 130012, People's Republic of China*
[33] *Johannes Gutenberg University of Mainz, Johann-Joachim-Becher-Weg 45, D-55099 Mainz, Germany*
[34] *Joint Institute for Nuclear Research, 141980 Dubna, Moscow region, Russia*
[35] *Justus-Liebig-Universitaet Giessen, II. Physikalisches Institut, Heinrich-Buff-Ring 16, D-35392 Giessen, Germany*
[36] *Lanzhou University, Lanzhou 730000, People's Republic of China*
[37] *Liaoning Normal University, Dalian 116029, People's Republic of China*
[38] *Liaoning University, Shenyang 110036, People's Republic of China*
[39] *Nanjing Normal University, Nanjing 210023, People's Republic of China*
[40] *Nanjing University, Nanjing 210093, People's Republic of China*
[41] *Nankai University, Tianjin 300071, People's Republic of China*
[42] *National Centre for Nuclear Research, Warsaw 02-093, Poland*
[43] *North China Electric Power University, Beijing 102206, People's Republic of China*
[44] *Peking University, Beijing 100871, People's Republic of China*
[45] *Qufu Normal University, Qufu 273165, People's Republic of China*
[46] *Shandong Normal University, Jinan 250014, People's Republic of China*
[47] *Shandong University, Jinan 250100, People's Republic of China*
[48] *Shanghai Jiao Tong University, Shanghai 200240, People's Republic of China*
[49] *Shanxi Normal University, Linfen 041004, People's Republic of China*
[50] *Shanxi University, Taiyuan 030006, People's Republic of China*
[51] *Sichuan University, Chengdu 610064, People's Republic of China*

[52] Soochow University, Suzhou 215006, People's Republic of China
[53] South China Normal University, Guangzhou 510006, People's Republic of China
[54] Southeast University, Nanjing 211100, People's Republic of China
[55] State Key Laboratory of Particle Detection and Electronics, Beijing 100049, Hefei 230026, People's Republic of China
[56] Sun Yat-Sen University, Guangzhou 510275, People's Republic of China
[57] Suranaree University of Technology, University Avenue 111, Nakhon Ratchasima 30000, Thailand
[58] Tsinghua University, Beijing 100084, People's Republic of China
[59] Turkish Accelerator Center Particle Factory Group, (A)Istinye University, 34010, Istanbul, Turkey; (B)Near East University, Nicosia, North Cyprus, Mersin 10, Turkey
[60] University of Chinese Academy of Sciences, Beijing 100049, People's Republic of China
[61] University of Groningen, NL-9747 AA Groningen, The Netherlands
[62] University of Hawaii, Honolulu, Hawaii 96822, USA
[63] University of Jinan, Jinan 250022, People's Republic of China
[64] University of Manchester, Oxford Road, Manchester, M13 9PL, United Kingdom
[65] University of Muenster, Wilhelm-Klemm-Strasse 9, 48149 Muenster, Germany
[66] University of Oxford, Keble Road, Oxford OX13RH, United Kingdom
[67] University of Science and Technology Liaoning, Anshan 114051, People's Republic of China
[68] University of Science and Technology of China, Hefei 230026, People's Republic of China
[69] University of South China, Hengyang 421001, People's Republic of China
[70] University of the Punjab, Lahore-54590, Pakistan
[71] University of Turin and INFN, (A)University of Turin, I-10125, Turin, Italy; (B)University of Eastern Piedmont, I-15121, Alessandria, Italy; (C)INFN, I-10125, Turin, Italy
[72] Uppsala University, Box 516, SE-75120 Uppsala, Sweden
[73] Wuhan University, Wuhan 430072, People's Republic of China
[74] Xinyang Normal University, Xinyang 464000, People's Republic of China
[75] Yantai University, Yantai 264005, People's Republic of China
[76] Yunnan University, Kunming 650500, People's Republic of China
[77] Zhejiang University, Hangzhou 310027, People's Republic of China
[78] Zhengzhou University, Zhengzhou 450001, People's Republic of China

[a] Also at the Moscow Institute of Physics and Technology, Moscow 141700, Russia
[b] Also at the Novosibirsk State University, Novosibirsk, 630090, Russia
[c] Also at the NRC "Kurchatov Institute", PNPI, 188300, Gatchina, Russia
[d] Also at Goethe University Frankfurt, 60323 Frankfurt am Main, Germany
[e] Also at Key Laboratory for Particle Physics, Astrophysics and Cosmology, Ministry of Education; Shanghai Key Laboratory for Particle Physics and Cosmology; Institute of Nuclear and Particle Physics, Shanghai 200240, People's Republic of China
[f] Also at Key Laboratory of Nuclear Physics and Ion-beam Application (MOE) and Institute of Modern Physics, Fudan University, Shanghai 200443, People's Republic of China
[g] Also at State Key Laboratory of Nuclear Physics and Technology, Peking University, Beijing 100871, People's Republic of China
[h] Also at School of Physics and Electronics, Hunan University, Changsha 410082, China
[i] Also at Guangdong Provincial Key Laboratory of Nuclear Science, Institute of Quantum Matter, South China Normal University, Guangzhou 510006, China
[j] Also at Frontiers Science Center for Rare Isotopes, Lanzhou University, Lanzhou 730000, People's Republic of China
[k] Also at Lanzhou Center for Theoretical Physics, Lanzhou University, Lanzhou 730000, People's Republic of China
[l] Also at the Department of Mathematical Sciences, IBA, Karachi , Pakistan
[m] Now at Zhejiang Jiaxing Digital City Laboratory Co., Ltd, Jiaxing 314051, People's Republic of China

(Dated: November 21, 2022)

# I. NORMALIZED DIFFERENTIAL CROSS SECTIONS OF THE $e^+e^- \to \pi^0 + X$ PROCESS

TABLE I. Summary of $N_{\pi^0}^{\text{obs}}$ in different momentum ranges at different c.m. energies, where the uncertainties are statistical.

| $p_{\pi^0}$ (GeV/$c$) | $\sqrt{s}$ = 2.2324 GeV | $\sqrt{s}$ = 2.4000 GeV | $\sqrt{s}$ = 2.8000 GeV | $\sqrt{s}$ = 3.0500 GeV | $\sqrt{s}$ = 3.4000 GeV | $\sqrt{s}$ = 3.6710 GeV |
|---|---|---|---|---|---|---|
| 0.00 − 0.10 | 1790 ± 171 | 1875 ± 166 | 1862 ± 49 | 6184 ± 363 | 642 ± 121 | 1296 ± 108 |
| 0.10 − 0.20 | 7894 ± 427 | 8144 ± 292 | 7530 ± 282 | 28454 ± 647 | 3150 ± 215 | 7588 ± 118 |
| 0.20 − 0.30 | 11640 ± 222 | 13428 ± 249 | 11952 ± 259 | 41689 ± 502 | 4470 ± 171 | 10986 ± 100 |
| 0.30 − 0.40 | 12659 ± 195 | 14872 ± 255 | 12872 ± 211 | 44503 ± 415 | 5080 ± 161 | 12117 ± 257 |
| 0.40 − 0.50 | 9690 ± 150 | 11416 ± 167 | 10425 ± 174 | 35120 ± 335 | 4071 ± 112 | 9405 ± 167 |
| 0.50 − 0.60 | 6534 ± 114 | 7776 ± 128 | 7082 ± 123 | 25612 ± 235 | 2954 ± 49 | 7125 ± 120 |
| 0.60 − 0.70 | 3735 ± 81 | 4695 ± 101 | 4598 ± 101 | 17164 ± 175 | 2066 ± 67 | 4975 ± 105 |
| 0.70 − 0.80 | 2135 ± 60 | 2764 ± 68 | 3047 ± 75 | 10830 ± 154 | 1440 ± 59 | 3529 ± 94 |
| 0.80 − 0.90 | 1350 ± 43 | 1596 ± 49 | 1871 ± 56 | 7077 ± 116 | 923 ± 43 | 2350 ± 71 |
| 0.90 − 1.00 | 949 ± 33 | 918 ± 34 | 1143 ± 42 | 4548 ± 90 | 545 ± 32 | 1591 ± 45 |
| 1.00 − 1.10 | − | 634 ± 28 | 727 ± 32 | 2884 ± 64 | 386 ± 24 | 981 ± 42 |
| 1.10 − 1.20 | − | − | 367 ± 24 | 1758 ± 56 | 273 ± 21 | 674 ± 36 |
| 1.20 − 1.30 | − | − | 269 ± 17 | 1010 ± 37 | 186 ± 17 | 494 ± 30 |
| 1.30 − 1.40 | − | − | − | 494 ± 28 | 129 ± 10 | 351 ± 23 |
| 1.40 − 1.50 | − | − | − | − | 69 ± 11 | 221 ± 15 |
| 1.50 − 1.60 | − | − | − | − | 32 ± 5 | 114 ± 12 |
| 1.60 − 1.70 | − | − | − | − | − | 59 ± 11 |

TABLE II. Summary of $f_{\pi^0}$ for different momentum ranges at different c.m. energies, where the uncertainties are statistical.

| $p_{\pi^0}$ (GeV/$c$) | $\sqrt{s}$ = 2.2324 GeV | $\sqrt{s}$ = 2.4000 GeV | $\sqrt{s}$ = 2.8000 GeV | $\sqrt{s}$ = 3.0500 GeV | $\sqrt{s}$ = 3.4000 GeV | $\sqrt{s}$ = 3.6710 GeV |
|---|---|---|---|---|---|---|
| 0.00 − 0.10 | 2.366 ± 0.034 | 2.349 ± 0.034 | 2.382 ± 0.039 | 2.389 ± 0.042 | 2.609 ± 0.048 | 2.555 ± 0.051 |
| 0.10 − 0.20 | 2.328 ± 0.016 | 2.403 ± 0.018 | 2.454 ± 0.019 | 2.577 ± 0.021 | 2.776 ± 0.023 | 2.708 ± 0.023 |
| 0.20 − 0.30 | 2.160 ± 0.010 | 2.197 ± 0.011 | 2.280 ± 0.012 | 2.372 ± 0.012 | 2.561 ± 0.014 | 2.497 ± 0.013 |
| 0.30 − 0.40 | 1.818 ± 0.007 | 1.866 ± 0.007 | 1.964 ± 0.007 | 2.030 ± 0.008 | 2.215 ± 0.009 | 2.188 ± 0.010 |
| 0.40 − 0.50 | 1.743 ± 0.006 | 1.799 ± 0.007 | 1.887 ± 0.007 | 1.941 ± 0.008 | 2.080 ± 0.009 | 2.096 ± 0.009 |
| 0.50 − 0.60 | 1.741 ± 0.008 | 1.770 ± 0.007 | 1.849 ± 0.008 | 1.907 ± 0.008 | 1.961 ± 0.009 | 2.028 ± 0.010 |
| 0.60 − 0.70 | 1.741 ± 0.009 | 1.788 ± 0.009 | 1.821 ± 0.009 | 1.872 ± 0.005 | 1.874 ± 0.010 | 1.964 ± 0.011 |
| 0.70 − 0.80 | 1.813 ± 0.012 | 1.815 ± 0.011 | 1.856 ± 0.010 | 1.882 ± 0.011 | 1.786 ± 0.011 | 1.912 ± 0.013 |
| 0.80 − 0.90 | 1.985 ± 0.016 | 1.923 ± 0.014 | 1.916 ± 0.013 | 1.934 ± 0.013 | 1.795 ± 0.012 | 1.918 ± 0.014 |
| 0.90 − 1.00 | 2.295 ± 0.022 | 2.124 ± 0.020 | 2.031 ± 0.016 | 1.987 ± 0.015 | 1.812 ± 0.014 | 1.906 ± 0.016 |
| 1.00 − 1.10 | − | 2.454 ± 0.027 | 2.138 ± 0.021 | 2.042 ± 0.017 | 1.855 ± 0.016 | 1.926 ± 0.017 |
| 1.10 − 1.20 | − | − | 2.354 ± 0.026 | 2.168 ± 0.024 | 1.967 ± 0.022 | 1.951 ± 0.019 |
| 1.20 − 1.30 | − | − | 2.637 ± 0.039 | 2.458 ± 0.033 | 2.092 ± 0.023 | 2.069 ± 0.023 |
| 1.30 − 1.40 | − | − | − | 2.451 ± 0.042 | 2.223 ± 0.028 | 2.064 ± 0.024 |
| 1.40 − 1.50 | − | − | − | − | 2.457 ± 0.039 | 2.241 ± 0.030 |
| 1.50 − 1.60 | − | − | − | − | 2.846 ± 0.058 | 2.478 ± 0.039 |
| 1.60 − 1.70 | − | − | − | − | − | 2.788 ± 0.036 |

TABLE III. Summary of normalized differential cross sections of the $e^+e^- \to \pi^0 + X$ process at different momentum ranges, where the first uncertainties are statistical and the second are systematic, respectively. Systematic uncertainties are regarded as uncorrelated between different momentum ranges except 2% of that due to the reconstruction of the photons.

| $p_{\pi^0}$ (GeV/$c$) | $\sqrt{s}$ = 2.2324 GeV | $\sqrt{s}$ = 2.4000 GeV | $\sqrt{s}$ = 2.8000 GeV | $\sqrt{s}$ = 3.0500 GeV | $\sqrt{s}$ = 3.4000 GeV | $\sqrt{s}$ = 3.6710 GeV |
|---|---|---|---|---|---|---|
| 0.00 − 0.10 | 0.522 ± 0.051 ± 0.121 | 0.467 ± 0.042 ± 0.065 | 0.543 ± 0.017 ± 0.127 | 0.535 ± 0.033 ± 0.099 | 0.534 ± 0.101 ± 0.258 | 0.482 ± 0.041 ± 0.141 |
| 0.10 − 0.20 | 2.263 ± 0.124 ± 0.213 | 2.075 ± 0.076 ± 0.211 | 2.261 ± 0.087 ± 0.390 | 2.656 ± 0.065 ± 0.203 | 2.789 ± 0.193 ± 0.306 | 2.987 ± 0.054 ± 0.577 |
| 0.20 − 0.30 | 3.097 ± 0.062 ± 0.240 | 3.128 ± 0.061 ± 0.098 | 3.334 ± 0.075 ± 0.188 | 3.581 ± 0.048 ± 0.282 | 3.651 ± 0.142 ± 0.242 | 3.988 ± 0.045 ± 0.437 |
| 0.30 − 0.40 | 2.834 ± 0.046 ± 0.087 | 2.943 ± 0.052 ± 0.169 | 3.093 ± 0.053 ± 0.103 | 3.272 ± 0.034 ± 0.119 | 3.588 ± 0.116 ± 0.190 | 3.854 ± 0.085 ± 0.211 |
| 0.40 − 0.50 | 2.081 ± 0.034 ± 0.046 | 2.178 ± 0.034 ± 0.048 | 2.407 ± 0.042 ± 0.086 | 2.468 ± 0.026 ± 0.086 | 2.700 ± 0.077 ± 0.150 | 2.866 ± 0.054 ± 0.087 |
| 0.50 − 0.60 | 1.401 ± 0.026 ± 0.032 | 1.460 ± 0.025 ± 0.036 | 1.603 ± 0.029 ± 0.057 | 1.769 ± 0.018 ± 0.039 | 1.847 ± 0.033 ± 0.070 | 2.101 ± 0.038 ± 0.064 |
| 0.60 − 0.70 | 0.801 ± 0.018 ± 0.023 | 0.890 ± 0.020 ± 0.025 | 1.024 ± 0.023 ± 0.070 | 1.164 ± 0.013 ± 0.054 | 1.234 ± 0.041 ± 0.062 | 1.420 ± 0.032 ± 0.045 |
| 0.70 − 0.80 | 0.477 ± 0.014 ± 0.014 | 0.532 ± 0.014 ± 0.019 | 0.692 ± 0.018 ± 0.063 | 0.738 ± 0.011 ± 0.069 | 0.820 ± 0.035 ± 0.100 | 0.981 ± 0.027 ± 0.071 |
| 0.80 − 0.90 | 0.330 ± 0.011 ± 0.026 | 0.326 ± 0.010 ± 0.015 | 0.439 ± 0.014 ± 0.043 | 0.496 ± 0.009 ± 0.050 | 0.528 ± 0.025 ± 0.076 | 0.655 ± 0.020 ± 0.062 |
| 0.90 − 1.00 | 0.268 ± 0.010 ± 0.032 | 0.207 ± 0.008 ± 0.029 | 0.284 ± 0.011 ± 0.031 | 0.327 ± 0.007 ± 0.046 | 0.315 ± 0.019 ± 0.054 | 0.441 ± 0.013 ± 0.065 |
| 1.00 − 1.10 | − | 0.165 ± 0.007 ± 0.036 | 0.190 ± 0.009 ± 0.024 | 0.213 ± 0.005 ± 0.038 | 0.228 ± 0.014 ± 0.043 | 0.275 ± 0.012 ± 0.065 |
| 1.10 − 1.20 | − | − | 0.106 ± 0.007 ± 0.019 | 0.138 ± 0.005 ± 0.024 | 0.171 ± 0.013 ± 0.026 | 0.191 ± 0.010 ± 0.041 |
| 1.20 − 1.30 | − | − | 0.087 ± 0.006 ± 0.043 | 0.090 ± 0.004 ± 0.022 | 0.124 ± 0.011 ± 0.028 | 0.149 ± 0.009 ± 0.036 |
| 1.30 − 1.40 | − | − | − | 0.044 ± 0.003 ± 0.018 | 0.091 ± 0.007 ± 0.023 | 0.105 ± 0.007 ± 0.035 |
| 1.40 − 1.50 | − | − | − | − | 0.054 ± 0.009 ± 0.016 | 0.072 ± 0.005 ± 0.030 |
| 1.50 − 1.60 | − | − | − | − | 0.029 ± 0.005 ± 0.011 | 0.041 ± 0.004 ± 0.013 |
| 1.60 − 1.70 | − | − | − | − | − | 0.024 ± 0.005 ± 0.015 |

## II. NORMALIZED DIFFERENTIAL CROSS SECTIONS OF THE $e^+e^- \to K_S^0 + X$ PROCESS

TABLE IV. Summary of $N_{K_S^0}^{\rm obs}$ in different momentum ranges at different c.m. energies, where the uncertainties are statistical.

| $p_{K_S^0}$ (GeV/$c$) | $\sqrt{s}$ = 2.2324 GeV | $\sqrt{s}$ = 2.4000 GeV | $\sqrt{s}$ = 2.8000 GeV | $\sqrt{s}$ = 3.0500 GeV | $\sqrt{s}$ = 3.4000 GeV | $\sqrt{s}$ = 3.6710 GeV |
|---|---|---|---|---|---|---|
| 0.00 − 0.10 | 48 ± 7 | 30 ± 6 | 27 ± 4 | 108 ± 13 | 9 ± 3 | 29 ± 7 |
| 0.10 − 0.20 | 271 ± 19 | 327 ± 22 | 258 ± 18 | 814 ± 38 | 68 ± 9 | 212 ± 17 |
| 0.20 − 0.30 | 501 ± 28 | 584 ± 30 | 579 ± 30 | 1739 ± 52 | 199 ± 18 | 371 ± 27 |
| 0.30 − 0.40 | 594 ± 31 | 743 ± 34 | 765 ± 35 | 2375 ± 66 | 285 ± 21 | 587 ± 33 |
| 0.40 − 0.50 | 552 ± 33 | 683 ± 35 | 721 ± 33 | 2468 ± 69 | 264 ± 20 | 596 ± 34 |
| 0.50 − 0.60 | 390 ± 25 | 511 ± 30 | 634 ± 33 | 2075 ± 62 | 258 ± 21 | 557 ± 29 |
| 0.60 − 0.70 | 273 ± 21 | 363 ± 25 | 416 ± 25 | 1613 ± 52 | 219 ± 17 | 511 ± 28 |
| 0.70 − 0.80 | 146 ± 15 | 221 ± 17 | 323 ± 21 | 1188 ± 42 | 149 ± 15 | 384 ± 24 |
| 0.80 − 0.90 | 137 ± 14 | 121 ± 14 | 192 ± 17 | 875 ± 35 | 120 ± 13 | 264 ± 21 |
| 0.90 − 1.00 | – | 128 ± 12 | 97 ± 12 | 596 ± 30 | 64 ± 10 | 222 ± 17 |
| 1.00 − 1.10 | – | – | 77 ± 10 | 351 ± 22 | 44 ± 7 | 145 ± 14 |
| 1.10 − 1.20 | – | – | 30 ± 6 | 196 ± 17 | 48 ± 8 | 100 ± 12 |
| 1.20 − 1.30 | – | – | – | 82 ± 12 | 17 ± 4 | 58 ± 9 |
| 1.30 − 1.40 | – | – | – | – | 16 ± 4 | 40 ± 8 |
| 1.40 − 1.50 | – | – | – | – | – | 31 ± 5 |

TABLE V. Summary of $f_{K_S^0}$ for different momentum ranges at different c.m. energies, where the uncertainties are statistical.

| $p_{K_S^0}$ (GeV/$c$) | $\sqrt{s}$ = 2.2324 GeV | $\sqrt{s}$ = 2.4000 GeV | $\sqrt{s}$ = 2.8000 GeV | $\sqrt{s}$ = 3.0500 GeV | $\sqrt{s}$ = 3.4000 GeV | $\sqrt{s}$ = 3.6710 GeV |
|---|---|---|---|---|---|---|
| 0.00 − 0.10 | 4.207 ± 0.108 | 3.952 ± 0.108 | 3.938 ± 0.096 | 4.200 ± 0.101 | 4.482 ± 0.136 | 4.093 ± 0.095 |
| 0.10 − 0.20 | 3.228 ± 0.038 | 3.264 ± 0.038 | 3.117 ± 0.035 | 3.183 ± 0.034 | 3.564 ± 0.051 | 3.353 ± 0.038 |
| 0.20 − 0.30 | 2.903 ± 0.038 | 3.026 ± 0.030 | 2.933 ± 0.026 | 2.922 ± 0.027 | 3.278 ± 0.034 | 3.174 ± 0.029 |
| 0.30 − 0.40 | 2.888 ± 0.034 | 2.925 ± 0.030 | 2.828 ± 0.023 | 2.836 ± 0.024 | 3.150 ± 0.033 | 2.917 ± 0.030 |
| 0.40 − 0.50 | 2.871 ± 0.051 | 2.951 ± 0.047 | 2.876 ± 0.030 | 2.751 ± 0.027 | 3.005 ± 0.042 | 2.910 ± 0.036 |
| 0.50 − 0.60 | 3.271 ± 0.071 | 3.106 ± 0.045 | 2.897 ± 0.041 | 2.758 ± 0.047 | 3.071 ± 0.040 | 2.814 ± 0.055 |
| 0.60 − 0.70 | 3.326 ± 0.073 | 3.333 ± 0.086 | 2.906 ± 0.051 | 2.777 ± 0.051 | 2.989 ± 0.054 | 2.977 ± 0.048 |
| 0.70 − 0.80 | 4.239 ± 0.121 | 3.744 ± 0.106 | 3.193 ± 0.056 | 2.886 ± 0.050 | 3.047 ± 0.050 | 2.950 ± 0.048 |
| 0.80 − 0.90 | 5.604 ± 0.174 | 3.998 ± 0.126 | 3.222 ± 0.076 | 3.205 ± 0.071 | 2.947 ± 0.059 | 2.971 ± 0.048 |
| 0.90 − 1.00 | – | 5.324 ± 0.192 | 4.054 ± 0.112 | 3.152 ± 0.076 | 3.038 ± 0.078 | 2.897 ± 0.058 |
| 1.00 − 1.10 | – | – | 4.505 ± 0.170 | 3.689 ± 0.115 | 3.271 ± 0.084 | 2.849 ± 0.068 |
| 1.10 − 1.20 | – | – | 5.132 ± 0.252 | 4.171 ± 0.157 | 3.618 ± 0.110 | 3.014 ± 0.074 |
| 1.20 − 1.30 | – | – | – | 4.643 ± 0.281 | 3.665 ± 0.183 | 3.150 ± 0.094 |
| 1.30 − 1.40 | – | – | – | – | 3.713 ± 0.261 | 3.483 ± 0.124 |
| 1.40 − 1.50 | – | – | – | – | – | 3.996 ± 0.266 |

TABLE VI. Summary of normalized differential cross sections of the $e^+e^- \to K_S^0 + X$ process at different momentum ranges, where the first uncertainties are statistical and the second are systematic, respectively. Systematic uncertainties are regarded as uncorrelated between different momentum ranges.

| $p_{K_S^0}$ (GeV/$c$) | $\sqrt{s}$ = 2.2324 GeV | $\sqrt{s}$ = 2.4000 GeV | $\sqrt{s}$ = 2.8000 GeV | $\sqrt{s}$ = 3.0500 GeV | $\sqrt{s}$ = 3.4000 GeV | $\sqrt{s}$ = 3.6710 GeV |
|---|---|---|---|---|---|---|
| 0.00 − 0.10 | 0.025 ± 0.004 ± 0.003 | 0.013 ± 0.002 ± 0.001 | 0.013 ± 0.002 ± 0.001 | 0.016 ± 0.002 ± 0.002 | 0.013 ± 0.005 ± 0.003 | 0.017 ± 0.004 ± 0.001 |
| 0.10 − 0.20 | 0.108 ± 0.007 ± 0.010 | 0.113 ± 0.008 ± 0.010 | 0.098 ± 0.007 ± 0.009 | 0.094 ± 0.004 ± 0.007 | 0.077 ± 0.011 ± 0.019 | 0.103 ± 0.008 ± 0.010 |
| 0.20 − 0.30 | 0.179 ± 0.009 ± 0.009 | 0.187 ± 0.010 ± 0.014 | 0.208 ± 0.011 ± 0.015 | 0.184 ± 0.006 ± 0.019 | 0.208 ± 0.019 ± 0.041 | 0.171 ± 0.012 ± 0.021 |
| 0.30 − 0.40 | 0.211 ± 0.010 ± 0.018 | 0.230 ± 0.011 ± 0.029 | 0.265 ± 0.012 ± 0.007 | 0.244 ± 0.007 ± 0.021 | 0.286 ± 0.021 ± 0.049 | 0.249 ± 0.014 ± 0.041 |
| 0.40 − 0.50 | 0.195 ± 0.010 ± 0.027 | 0.214 ± 0.011 ± 0.020 | 0.254 ± 0.012 ± 0.009 | 0.246 ± 0.007 ± 0.009 | 0.253 ± 0.019 ± 0.036 | 0.252 ± 0.015 ± 0.042 |
| 0.50 − 0.60 | 0.157 ± 0.010 ± 0.005 | 0.168 ± 0.010 ± 0.017 | 0.225 ± 0.012 ± 0.029 | 0.207 ± 0.007 ± 0.011 | 0.252 ± 0.021 ± 0.025 | 0.228 ± 0.012 ± 0.036 |
| 0.60 − 0.70 | 0.112 ± 0.008 ± 0.017 | 0.128 ± 0.009 ± 0.007 | 0.148 ± 0.009 ± 0.006 | 0.162 ± 0.006 ± 0.014 | 0.209 ± 0.017 ± 0.019 | 0.221 ± 0.012 ± 0.034 |
| 0.70 − 0.80 | 0.076 ± 0.008 ± 0.004 | 0.088 ± 0.007 ± 0.007 | 0.126 ± 0.009 ± 0.013 | 0.124 ± 0.005 ± 0.006 | 0.145 ± 0.015 ± 0.011 | 0.165 ± 0.010 ± 0.015 |
| 0.80 − 0.90 | 0.095 ± 0.010 ± 0.006 | 0.051 ± 0.006 ± 0.005 | 0.076 ± 0.007 ± 0.005 | 0.102 ± 0.005 ± 0.006 | 0.113 ± 0.012 ± 0.005 | 0.114 ± 0.009 ± 0.015 |
| 0.90 − 1.00 | – | 0.072 ± 0.007 ± 0.008 | 0.048 ± 0.006 ± 0.005 | 0.068 ± 0.004 ± 0.005 | 0.062 ± 0.010 ± 0.007 | 0.093 ± 0.007 ± 0.005 |
| 1.00 − 1.10 | – | – | 0.043 ± 0.006 ± 0.005 | 0.047 ± 0.003 ± 0.008 | 0.046 ± 0.008 ± 0.009 | 0.060 ± 0.006 ± 0.003 |
| 1.10 − 1.20 | – | – | 0.019 ± 0.004 ± 0.002 | 0.030 ± 0.003 ± 0.007 | 0.055 ± 0.009 ± 0.014 | 0.044 ± 0.005 ± 0.003 |
| 1.20 − 1.30 | – | – | – | 0.014 ± 0.002 ± 0.006 | 0.020 ± 0.005 ± 0.003 | 0.026 ± 0.004 ± 0.002 |
| 1.30 − 1.40 | – | – | – | – | 0.019 ± 0.005 ± 0.004 | 0.020 ± 0.004 ± 0.004 |
| 1.40 − 1.50 | – | – | – | – | – | 0.018 ± 0.003 ± 0.005 |
